# Supplementary material for: Precise Task Formalization Matters in Winograd Schema Evaluations
Source: arXiv:2010.04043 source file (2020-10-08)
Supplement: Supplementary file 1 [file appendices.tex]

\begin{appendices}
\section{Winogrande}
\label{appendix:A}

\begin{table}[h]
    \centering
    \resizebox{.45\textwidth}{!}{
    \begin{tabular}{l l l l}
        \toprule
        Formalization & Top & 3\textsuperscript{rd} Quartile & Difference\\
        \midrule
        MC-MLM          & 69.5\% & 67.5\% & 1.9\% \\
        MC-SENT         & 68.0\% & 53.1\% & 14.8\%\\
        MC-SENT-PAIR    & 66.4\% & 53.9\% & 12.5\%\\
        MC-SENT-PLOSS   & 54.5\% & 53.0\% & 1.6\% \\
        P-SENT          & 63.2\% & 50.4\% & 12.8\% \\
        P-SPAN          & 67.9\% & 65.9\% & 1.9\% \\
        \bottomrule
    \end{tabular}}
    % \caption{Statistics of validation accuracy. Difference is between top and 3\textsuperscript{rd} quartile values. Test results are from an ensemble of top 5 models.}
    \caption{Statistics of validation accuracy. Difference is between top and 3\textsuperscript{rd} quartile values.}
    \label{tab:stats}
\end{table}

\begin{figure*}[t]
    \centering
    \includegraphics[width=0.9\textwidth]{figures/winogrande_violin.pdf}
    \caption{Boxplot of validation accuracy from 60 runs on WinoGrande. The red line marks the median number and higher edge of the rectangle marks the 3\textsuperscript{rd} quartile. The numbers indicate the 3\textsuperscript{rd} quartile values.}
    \label{fig:results}
\end{figure*}
\end{appendices}
